# Supplementary material for: Computationally efficient joint coordination of multiple electric vehicle charging points using reinforcement learning
Source: arXiv:2203.14078 source file (2022-03-26)
Supplement: Supplementary file 1 [file appendix.tex]

%%%%%%%%%%%%%%%%%%%%%%%%%%%%%%%%%%%%%%%%%%%%%%%%%%%%%
\section{My Appendix}
%%%%%%%%%%%%%%%%%%%%%%%%%%%%%%%%%%%%%%%%%%%%%%%%%%%%
Add info in appendix
